# Supplementary material for: Alternating Updates for Efficient Transformers
Source: arXiv:2301.13310 source file (2023-10-03)
Supplement: Supplementary file 1 [file analysis.tex]

\section*{Proofs of the theoretical statements in Sec.~\ref{sec:analysis}}

Recall from Sec.~\ref{sec:analysis} that we consider two sentences $s_1, s_2$ of the same length $l$ that have $f$ fraction of wordpieces in common.
\lookupefficiency
\begin{proof}
For the first statement, we observe that the buckets in Spherical LSH correspond to the Voronoi regions formed by the randomly chosen set of points in $\mathbb{R}^d$. If we consider the Softmax routing matrix $W$ from Sec.~\ref{sec:routing-functions} to be random (see~\cite{andoni2015optimal} for details) and the rows to be of unit norm, then the experts' dot row-wise product with the top-1 routing will correspond to picking the expert whose routing vector is closest in angle to the input vector~\cite{andoni2015practical}. Min-hash involves hashing the universe of elements from which the sets are constructed randomly into some interval in the real line, and hashing a set to the element that has the smallest value on the real line. Thus each element can be viewed as a bucket. If we use the Jaccard simlarity measure for comparing sets (for two sets $A,B$ it is given by $\mathrm{sim}(A,B) = |A \cap B|/|A \cup B|$) then this hash function ensures that two sets $A,B$ will hash to the same bucket with probability equal to $\mathrm{sim}(A,B)$. Note that this same property holds for Token-ID lookup (Sec.~\ref{sec:routing-functions}) as each token at any layer is hashed to an expert specific to that token. In this sense, Min-hash LSH corresponds to Token-ID lookup.

For the second statement, we consider the setting of the theorem where we have two sentences $s_1,s_2$ of equal length and a fraction $f$ of wordpieces in common. Let us evaluate the probability of routing a certain token to the expert at some intermediate layer. Note that at intermediate layers we can assume that sufficient mixing has happened between the token due to self-attention modules. For simplicity, we can view this mixing as averaging the value of all the token embeddings. Since the initial wordpiece embeddings are random, after averaging the dot product between the two averages will be $f$ and so the distance between them will be $\mathcal O (\sqrt{1- f})$. On the other hand, if we take two sentences with no tokens in common the distance between them will be $\mathcal O(1)$.

An appropriate implementation of hyperplane LSH~\cite{datar2004locality} has the property $c = \mathcal O(1 / \sqrt{1 - f})$ and $\rho = \mathcal O(1/c) = \mathcal O (\sqrt{1 - f})$. With $n$ experts (buckets), this yields a collision probability of $n^{- \mathcal O(\sqrt{1 - f})}$ for the set of experts corresponding to the two similar sentences. Spherical LSH has the improved property that $\rho = \mathcal O (1 / c^2)$, which yields $ n^{-\mathcal O(1 - f)}$ for the collision probability based on the analysis above. For Min-hash, we know from the above that the probability that two sets $A$ and $B$ hash to the same bucket is equal to $\mathrm{sim}(A,B)$. This corresponds to the fraction of overlapping wordpieces in two sentences $s_1$ and $s_1$, hence the fraction of experts for which there is a collision is $f$. This proves the second statement of the theorem.

The third statement follows immediately from the second one, where the most efficient lookup is considered to be the one that has the highest probability of collision of two similar sentences. Hence, for large $n$ and small $f$, the order of efficacy is
$$
f \ge n^{- \mathcal O(1 - f)} \ge  n^{- \mathcal O(\sqrt{1 - f})}.
$$
This concludes the proof of the theorem.
\end{proof}

\embeddinglookup
\begin{proof}
% \cb{The proof is the same as the proof sketch in the main paper. Can we add more details here? Should be ok for now I guess and could do later if accepted? -- Rina; Sounds good - Cenk}
We consider two architectures that implement the embedding lookup in the two distinct ways and an input $(u, q)$ with ground truth score $\dotp{\Psi(u)}{\Phi(q)}$, where $\Psi(u)$ maps $u$ to a $d$-dimensional feature vector and $\Phi(q)$ is a non-linear transformation of $q$ that can be implemented by a deep network of width $d$. The first architecture combines the lookup $\Psi(u)$ with $q$ (by a weighted sum) and feeds into the network as input; the second architecture in addition feeds the embedding output of $u$ to all the layers of the network instead of only the lowest layer. The second architecture can store $\Psi(u)$ in the table and feed it directly to the output layer (which produces $\Phi(q)$) to obtain the result $\dotp{\Psi(u)}{\Phi(q)}$ using width $d$. On the other hand, for the first architecture the entropy of the information carried up the layers is at least $2d$ assuming $u$ and $q$ are random and not correlated, and so the width of the network needs to be $2d$.
\end{proof}
