# Supplementary material for: Alternating Updates for Efficient Transformers
Source: arXiv:2301.13310 source file (2023-10-03)
Supplement: Supplementary file 2 [file supplement.tex]

% TODO: 
% \begin{enumerate}
%     \item Full proofs and additional LSH details
%     \item Experimental details (e.g., explain what rank means, computation of additional parameters used, number of experts = 1, etc.)
%     \item Rank x buckets sweeps for base and large for LSH and token-routing as well
%     \item Fine-tuning experiments (super-glue, etc.)?
% \end{enumerate}

\section*{Supplementary Material for \textit{Efficient, High-capacity Transformers via Alternating Updates}}
In this supplementary, we present the full proofs of the theoretical statements in the main paper, details of the experimental evaluations, and additional empirical results.

\section*{Additional experiment setup details}
\label{sec:exp_setup}

\subsection*{Details of the T5 experiments}
%We train the T5 models for $100k$ steps\cb{? The main paper says 500k} \cb{TODO: Additional details here. Dropout, etc.} \xw{For the alternating updates experiments, we pretrain for 500k steps, and finetune for 50k steps; for the comparison of softmax, token memory, etc, we pretrain for 100k steps since it would take too long for 500k}.

% We evaluated our techniques on the T5 language models \cite{raffel2020exploring}. Specifically, we use the T5 version 1.1 models with gated GELU feedforward network and pre layernorm. The models are implemented on top of the T5X \cite{roberts2022t5x} code base. During pretraining, we use 256 batch size, Adafactor optimizer \cite{shazeer2018adafactor} with base learning rate $1.0$ and reciprocal square-root decay with $10000$ warmup steps, and zero dropout. During finetuning, we use 256 batch size, Adafactor optimizer with constant learning rate of $0.001$ and $0.1$ dropout. Unless explicited mentioned, we pretrain for $500,000$ steps and finetune for $50,000$ steps.

\subsection*{Details of the partial expert computation}
For all experiments, we used single partial expert lookup, i.e., $k = 1$ in SMoE terminology and added the the output of the partial expert to the output of the main expert. Throughout the paper, buckets are synonymous with partial experts. In our experiments we defined each partial expert as a FF network composed of two matrices $U, V \in \mathbb{R}^{d_\mathrm{in} \times \mathrm{rank}}$, where $d_\mathrm{in}$ is the embedding dimension of the input to the partial expert and $\mathrm{rank}$ is a configurable parameter that controls the width of the expert. The output for a $d_\mathrm{in}$-dimensional input $x$ is computed as $V \phi(U^T x)$ where $\phi(\cdot)$ is the nonlinearity. In this paper, we used the ReLU function for $\phi$, i.e., $\phi(x) = \max \{0, x\}$ entrywise. Note that adding $\mathrm{buckets}$ experts, each with rank $\mathrm{rank}$ adds a total of $2 \max  \{\mathrm{rank}, 1\} * \mathrm{buckets} * d_\mathrm{in}$ parameters to the network\footnote{We ignore the $d_\mathrm{in}$ factor when comparing various routing functions since this is universally present regardless of the partial experts configuration.}. The matrices were initialized according to LeCun normal initialization~\cite{lecun2012efficient}.

\subsection*{Softmax Routing}
For softmax routing, we used the simplified implementation of the top-1 routing of~\cite{fedus2021switch}. For sake of fair comparisons with other lookup methods that do not require load balancing, we did not consider an explicit technique for load balancing such as load balancing loss~\cite{fedus2021switch} or router z loss~\cite{zoph2022designing} due to the additional hyperparameters that they introduce. We use multiplicative jitter noise sampled from a uniform distribution over $[1 - \varepsilon, 1 + \varepsilon]^{d_\mathrm{in}}$~\cite{zoph2022designing,fedus2021switch} with $\varepsilon = 0.01$. The router matrix $W$ was initialized by drawing from a zero mean Normal distribution with standard deviation $2 \times 10^{-2}$.

\section*{Additional experiment results}
\label{sec:exp_results}

\subsubsection*{Additional experiments for memory consumption methods}
We provide additional experiments for memory consumption methods comparison. In section~\ref{sec:altup_results}, we presented the comparison on the T5 version 1.1 base size model. Here we present the results for T5 version 1.1 small and large size models in Table~\ref{table:altup_ablation_sl}. We observe the Prediction-Compute-Correct algorithm with \emph{same} and \emph{alternating} block selection methods outperforms the summation method. For the small models, \emph{same} block selection method performs better in most tasks, while for large models, \emph{alternating} block selection method performs better in most tasks.

\begin{table}
    
    \scalebox{0.85}{
    \begin{tabular}{@{}lcccc@{}}
    \toprule
    \multirow{2}{*}{\textbf{Model}} & {\textbf{Pretrain}} & {\textbf{Finetune}} & {\textbf{Finetune}} & {\textbf{Finetune}} \\
     & \textbf{accuracy} & \textbf{GLUE} & \textbf{SG} &\textbf{SQuAD (EM/F1)} \\
    \midrule
    S &    $61.21$ & $75.83$ & $59.52$ & $76.44/84.97$ \\
    S + Sum & $61.67$ & $77.54$ & $59.63$ & $75.06/83.82$\\
    S + SameUp &    $\mathbf{61.91}$ & $\mathbf{77.75}$ & $\mathbf{60.81}$ & $76.85/85.51$ \\
    S + AltUp & $61.86$ & $76.82$ & $59.60$ & $\mathbf{77.51/85.79}$\\
    \bottomrule
    \end{tabular}}
    \scalebox{0.85}{
    \begin{tabular}{@{}lcccc@{}}
    \toprule
    \multirow{2}{*}{\textbf{Model}} & {\textbf{Pretrain}} & {\textbf{Finetune}} & {\textbf{Finetune}} & {\textbf{Finetune}} \\
     & \textbf{accuracy} & \textbf{GLUE} & \textbf{SG} &\textbf{SQuAD (EM/F1)} \\
    \midrule
    L &    $69.13$ & $87.23$ & $81.21$ & $86.77/93.56$ \\
    L + Sum & $69.09$ & $86.18$ & $78.93$ & $86.19/93.08$\\
    L + SameUp &    $\mathbf{69.45}$ & $87.95$ & $82.72$ & $\mathbf{87.65}/ 94.13$ \\
    L + AltUp & $69.32$ & $\mathbf{88.20}$ & $\mathbf{82.75}$ & $87.58/\mathbf{94.27}$\\
    \bottomrule
    \end{tabular}}
    \caption{Comparison of memory consumption methods. T5 version 1.1 small (S) and large (L) models, with different memory consumption methods: summation (Sum), Predict-Compute-Correct with ``same" block selection (SameUp), and Predict-Compute-Correct with ``alternating" block selection (AltUp).}
    \label{table:altup_ablation_sl}
    %\vspace{-3mm}
\end{table}

\subsubsection*{Additional experiments for different memory sizes}

We report the performance of T5 version 1.1 small and large models with different memory sizes in Table~\ref{table:altup_scaleup_sl}. We observe that for the large models, the trend is similar to the T5 base sized model, i.e. more memory improves both pretrain and finetune quality; while for the small model, more memory improves pretrain quality, but the finetune quality doesn't improve, likely due to overfitting from the additional parameters. 
