# Supplementary material for: Alternating Updates for Efficient Transformers
Source: arXiv:2301.13310 source file (2023-10-03)
Supplement: Supplementary file 3 [file experiment_results.tex]

\section*{Additional experiment results}
\label{sec:exp_results}

\subsubsection*{Additional experiments for memory consumption methods}
We provide additional experiments for memory consumption methods comparison. In section~\ref{sec:altup_results}, we presented the comparison on the T5 version 1.1 base size model. Here we present the results for T5 version 1.1 small and large size models in Table~\ref{table:altup_ablation_sl}. We observe the Prediction-Compute-Correct algorithm with \emph{same} and \emph{alternating} block selection methods outperforms the summation method. For the small models, \emph{same} block selection method performs better in most tasks, while for large models, \emph{alternating} block selection method performs better in most tasks.

\begin{table}
    
    \scalebox{0.85}{
    \begin{tabular}{@{}lcccc@{}}
    \toprule
    \multirow{2}{*}{\textbf{Model}} & {\textbf{Pretrain}} & {\textbf{Finetune}} & {\textbf{Finetune}} & {\textbf{Finetune}} \\
     & \textbf{accuracy} & \textbf{GLUE} & \textbf{SG} &\textbf{SQuAD (EM/F1)} \\
    \midrule
    S &    $61.21$ & $75.83$ & $59.52$ & $76.44/84.97$ \\
    S + Sum & $61.67$ & $77.54$ & $59.63$ & $75.06/83.82$\\
    S + SameUp &    $\mathbf{61.91}$ & $\mathbf{77.75}$ & $\mathbf{60.81}$ & $76.85/85.51$ \\
    S + AltUp & $61.86$ & $76.82$ & $59.60$ & $\mathbf{77.51/85.79}$\\
    \bottomrule
    \end{tabular}}
    \scalebox{0.85}{
    \begin{tabular}{@{}lcccc@{}}
    \toprule
    \multirow{2}{*}{\textbf{Model}} & {\textbf{Pretrain}} & {\textbf{Finetune}} & {\textbf{Finetune}} & {\textbf{Finetune}} \\
     & \textbf{accuracy} & \textbf{GLUE} & \textbf{SG} &\textbf{SQuAD (EM/F1)} \\
    \midrule
    L &    $69.13$ & $87.23$ & $81.21$ & $86.77/93.56$ \\
    L + Sum & $69.09$ & $86.18$ & $78.93$ & $86.19/93.08$\\
    L + SameUp &    $\mathbf{69.45}$ & $87.95$ & $82.72$ & $\mathbf{87.65}/ 94.13$ \\
    L + AltUp & $69.32$ & $\mathbf{88.20}$ & $\mathbf{82.75}$ & $87.58/\mathbf{94.27}$\\
    \bottomrule
    \end{tabular}}
    \caption{Comparison of memory consumption methods. T5 version 1.1 small (S) and large (L) models, with different memory consumption methods: summation (Sum), Predict-Compute-Correct with ``same" block selection (SameUp), and Predict-Compute-Correct with ``alternating" block selection (AltUp).}
    \label{table:altup_ablation_sl}
    %\vspace{-3mm}
\end{table}

\subsubsection*{Additional experiments for different memory sizes}

We report the performance of T5 version 1.1 small and large models with different memory sizes in Table~\ref{table:altup_scaleup_sl}. We observe that for the large models, the trend is similar to the T5 base sized model, i.e. more memory improves both pretrain and finetune quality; while for the small model, more memory improves pretrain quality, but the finetune quality doesn't improve, likely due to overfitting from the additional parameters. 
